# Supplementary material for: sCWatter: Open source coupled wave scattering simulation for spectroscopy and microscopy
Source: arXiv:2404.07293 source file (2024-04-10)
Supplement: Supplementary file 1 [file homogeneous_supplement.tex]

\subsection{Homogeneous Samples}
\david{If we keep this section, replace F with R. Remove B (because we use it later)}
A homogeneous layered sample provides a simple case, since the model can be characterized with one spatial frequency ($M=1$) and the electric field (Equation \ref{eqn:e_from_p}) simplifies to:
\begin{equation*}
    \mathbf{E}(\mathbf{r}, z) = \mathbf{P}(\mathbf{s}, z) \textup{exp}(ik\mathbf{s}\cdot\mathbf{r})
\end{equation*}
We define the field propagating into the sample from the boundary interfaces $z_0$ and $z_L$ as:
\begin{itemize}
    \item $\check{\mathbf{F}}(\mathbf{s})$ are the coefficients of the internal field transmitted into the sample from the top ($z_0$).
    \item $\hat{\mathbf{F}}(\mathbf{s})$ are the coefficients of the internal field reflected into the sample from $z_L$.
\end{itemize}

$\check{\mathbf{F}}(\mathbf{s})$ and $\hat{\mathbf{F}}(\mathbf{s})$ provide sufficient information to calculate the field anywhere within the sample\cite{davis2010theory}. Any point outside of the sample can be calculated using $\bar{\mathbf{P}}(\mathbf{s})$, $\hat{\mathbf{P}}(\mathbf{s})$, and $\check{\mathbf{P}}(\mathbf{s})$ (Section \ref{sec:scattered_fields}). A linear system is built to solve for $\hat{\mathbf{P}}(\mathbf{s})$, $\check{\mathbf{P}}(\mathbf{s})$, $\check{\mathbf{F}}(\mathbf{s})$, and $\hat{\mathbf{F}}(\mathbf{s})$ given the incident field $\bar{\mathbf{P}}(\mathbf{s})$ using Maxwell's equations:
\begin{equation}
    \triangledown  \cdot \mathbf{E}(\mathbf {r}, t)=\frac{\rho}{\epsilon_0}
\label{eqn:gauss_law}
\end{equation}
\begin{equation}
    \triangledown  \times \mathbf{E}(\mathbf {r}, t)=-\frac{\partial \mathbf{B}}{\partial t}
\label{eqn:faraday_law}
\end{equation}
\begin{equation}
    \triangledown  \times \mathbf{H}(\mathbf {r}, t)= \mathbf J+\frac{\partial \mathbf{D}}{\partial t}
\label{eqn:Ampere_law}
\end{equation}
where $\mathbf E$ is the electric field, $\rho$ is the charge density and $\epsilon_0$ is the vacuum permittivity for the equation \ref{eqn:gauss_law}, and $\mathbf{H}$ is the magnetic field for the equation \ref{eqn:faraday_law}. This provides a set of $12$ constraints to solve the field at the boundary. 

\subsubsection{Gauss' Law (4M)}

Assuming that the sample does not contain an electrical charge, the charge density $\rho$ is zero. Gauss' Law (Equation \ref{eqn:gauss_law}) at each layer boundary can be written as:
\begin{equation}
    \frac{\partial\mathbf{P}}{\partial x} + \frac{\partial\mathbf{P}}{\partial y} + \frac{\partial\mathbf{P}}{\partial z} = 
    \mathbf{s}^T \mathbf{P} = 0
\end{equation}
which is simplified for the upward field and the downward field for a single coefficient ($M=1$) as below:
\begin{equation}
\mathbf{s}_z \cdot \check{\mathbf{P}}(\mathbf{s}_z) = 0
%s_x(u, v)\check{P}_{x}(s_x(u, v)) + s_y(u, v)\check{P}_{y}(s_y(u, v)) + s_z(u, v)\check{P}_{z}(s_z(u, v)) = 0 
\label{eqn:gauss-1}
\end{equation}
\begin{equation}
\mathbf{s}_z \cdot \hat{\mathbf{P}}(\mathbf{s}_z) = 0
%s_x(u, v)\hat{P}_{x}(s_x(u, v)) + s_y(u, v)\hat{P}_{y}(s_y(u, v) + s_z(u, v)\hat{P}_{z}(s_z(u, v)) = 0
\label{eqn:gauss-2}
\end{equation}
where $\mathbf{P}(\mathbf{s}) = [ P_{x}, P_{y}, P_{z}]^T$ is the field vector, and $\mathbf{s}_z=[\mathbf s ^T, s_z] = [s_x, s_y, s_z]^T$ are the components of the Fourier coefficients of the propagation direction vector (Equations \ref{eqn:direction_vector} and \ref{eqn:direction_vector_z}).

Similarly, Gauss' Law provides $6M$ constraints for $\mathbf F$, $3M$ of which are for upward $\hat{\mathbf F}$ and $3M$ of which are for downward $\check{\mathbf F}$. For a homogeneous sample ($M=1$), Equation \ref{eqn:gauss_law} are the only 4 constraints:
\begin{equation}
\mathbf{s}_m \cdot \hat{\mathbf{P}}(\mathbf{s}_m) =
s_{m,x}\hat{P}_{x}(\mathbf{s}_m) + s_{m,y}\hat{P}_{y}(\mathbf{s}_m) + s_{m,z}\hat{P}_{z}(\mathbf{s}_m) = 0
\label{eqn:gauss1}
\end{equation}
\begin{equation}
\mathbf{s}_m \cdot \check{\mathbf{P}}(\mathbf{s}_m) = s_{m,x}\check{P}_{x}(\mathbf{s}_m) + s_{m,y}\check{P}_{y}(\mathbf{s}_m) + s_{m,z}\check{P}_{z}(\mathbf{s}_m) = 0 
\label{eqn:gauss2}
\end{equation}
\begin{equation}
\mathbf{s}_m \cdot \check{\mathbf{F}}(\mathbf{s}_m) = s_{m,x}\check{F}_{x}(\mathbf{s}_m) + s_{m,y}\check{F}_{y}(\mathbf{s}_m) + s_{m,z}\check{F}_{z}(\mathbf{s}_m) = 0 
\label{eqn:gauss3}
\end{equation}
\begin{equation}
\mathbf{s}_m \cdot \hat{\mathbf{F}}(\mathbf{s}_m) =
s_{m,x}\hat{F}_{x}(\mathbf{s}_m) + s_{m,y}\hat{F}_{y}(\mathbf{s}_m) + s_{m,z}\hat{F}_{z}(\mathbf{s}_m) = 0
\label{eqn:gauss4}
\end{equation}

\subsubsection{Boundary conditions (8M)}
Faraday's Law (Equation \ref{eqn:faraday_law}) and Ampere's Law (Equation \ref{eqn:Ampere_law}) require that the electric and magnetic fields at any boundary are continuous. Therefore the difference between the reflected and transmitted electric and magnetic fields must be zero:
\begin{equation}
\mathbf{E}_1 - \mathbf{E}_2 = 0
\label{eqn:boundary_1}
\end{equation}
\begin{equation}
\mathbf{H}_1 - \mathbf{H}_2 = 0
\label{eqn:boundary_2}
\end{equation}

\begin{figure}[tb]\centering
\includegraphics[width=\linewidth]{figures/homogeneous_matrix.pdf}
\caption{The electric field vector $P$ at the homogeneous boundaries is calculated by solving the linear system. For the $12$ linearly independent conditions, $4$ linearly independent conditions are provided by Gauss' Equations (Equations \ref{eqn:gauss1} - \ref{eqn:gauss4}), and $8$ by the boundary equations (Equations \ref{eqn:boundary1} - \ref{eqn:boundary8}).}
\label{fig:linear_system_homo}
\end{figure} 

For a homogeneous sample (M=1), we represent the refractive index for the sample layer as $n_1$. The propagation direction is $\mathbf s = [s_x,s_y]^T$. To enforce the continuity of the transverse components of $\mathbf{E}(\mathbf{r}, z)$ and $\mathbf{H}(\mathbf{r}, z)$ across layer boundaries (Equations \ref{eqn:boundary_1} and \ref{eqn:boundary_2}), the boundary conditions at $z_0$ provide $4$ constraints:
\begin{equation}
\begin{aligned}
\bar P_{x} G\left[s_z(\hat {n}), z_0, \bar z\right] + \hat P_{x} =  \check F_{x} + \hat F_{x}G\left[-s_z(n_1), z_0, z_L\right]
\end{aligned}
\label{eqn:boundary1}
\end{equation}
\begin{equation}
\begin{aligned}
\check P_{y} G\left[s_z(\hat {n}), z_0, \bar z\right] + \hat P_{y} = \check F_{y} + \hat F_{y}G\left[-s_z(n_1), z_0, z_L\right]
\end{aligned}
\label{eqn:boundary2}
\end{equation}
\begin{equation}
\begin{aligned}
&\left(s_y\bar P_{z} -s_z(\hat {n})\bar P_{y}\right) G\left[s_z(\hat {n}), z_0, \bar z\right] +
s_y  \hat P_{z}+s_z(\hat {n})\hat P_{y} \\&=  s_y\check F_{z} - s_z(n_1)\check F_{y} +\left(s_y \hat F_{z}+ s_z(n_1)\hat F_{y}\right)G\left[-s_z(n_1), z_0, z_L\right]
\end{aligned}
\label{eqn:boundary3}
\end{equation}
\begin{equation}
\begin{aligned}
&\left(s_z(\hat {n})\bar P_{x}-s_x\bar P_{z}\right)G\left[s_z(\hat {n}), z_0, \bar z\right]
-s_z(\hat {n})\hat P_{x}-s_x\hat P_{z} \\&= s_z(n_1)\check F_{x} - s_x\check F_{z} +\left(-s_z(n_1)\hat F_{z} - s_x\hat F_{z}\right)G\left[-s_z(n_1), z_0, z_L\right]
\end{aligned}
\label{eqn:boundary4}
\end{equation}
The boundary conditions at $z_L$ provide the final $4$ constraints:
\begin{equation}
\begin{aligned}
\check F_x G\left[s_z(n_1), z_L, z_0\right] + \hat F_{x} = \check P_{x}
\end{aligned}
\label{eqn:boundary5}
\end{equation}
\begin{equation}
\begin{aligned}
\check F_y G\left[s_z(n_1), z_L, z_0\right] + \hat F_{y}= \check P_{y}
\end{aligned}
\label{eqn:boundary6}
\end{equation}
\begin{equation}
\begin{aligned}
\left(s_y\check F_{z} - s_z(n_1)\bar F_{y}\right) &G\left[s_z(n_1), z_L, z_0\right] \\ 
&+s_y  \hat F_{z}+ s_z(n_1)\hat F_{y} = s_y\check P_{z}-  s_z(\check {n})\check P_{y}
\end{aligned}
\label{eqn:boundary7}
\end{equation}
\begin{equation}
\begin{aligned}
\left( s_z( n_1)\check F_{x}-s_x\check F_{z}\right)& G\left[s_z(n_1), z_L, z_0\right]  \\
&- s_z(n_1)\hat F_{x}-s_x\hat F_{z} = s_z(\check {n})\check P_{x} - s_x\check P_{z}
\end{aligned}
\label{eqn:boundary8}
\end{equation}
The linear system (Figure \ref{fig:linear_system_homo}) are constructed by Equations \ref{eqn:gauss1}-\ref{eqn:gauss4}, and \ref{eqn:boundary1}-\ref{eqn:boundary8}.
